# Supplementary material for: The Bias is in the Details: An Assessment of Cognitive Bias in LLMs
Source: arXiv:2509.22856 source file (2025-09-26)
Supplement: Supplementary file 1 [file prompts.tex]

\subsection{System Prompt}

In addition to the augmented prompts generated by our evaluation pipeline, we include a single system prompt to ground each model in a multiple-choice evaluation setting:
